# Supplementary material for: Benchmarking Sequential Visual Input Reasoning and Prediction in Multimodal Large Language Models
Source: arXiv:2310.13473 source file (2023-10-20)
Supplement: Supplementary file 1 [file crop_appendix_examples_abstrct.1.pdf]

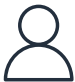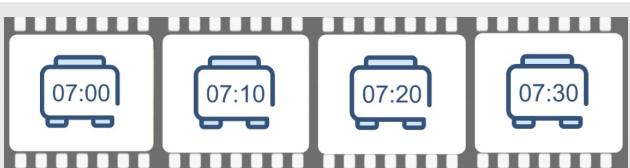

**User:** As an artificial intelligence assistant capable of interpreting visual information, you have seen an ordered sequence of {} individual images, arranged in chronological order from left to right. There is a pattern in these images. Your task is to tell me what this pattern is and predict what will happen to the upcoming image according to this pattern. Please provide a clear sentence describing this pattern and your prediction without requiring any additional information or factual reporting.

**LLaVA:** The pattern observed in the images is that each one displays a progressive time, with the leftmost image showing a time of 7:55, the second one showing 8:00, the third one showing 8:05, and the fourth one showing 8:10. Based on this pattern, it can be predicted that the upcoming image will display a time of 8:15.

**GPT-4:** 1. LogicalConsistency: score: 0. reason: The model's response does not match the pattern described in <P>. The times given by the model are different from those provided in <P>. 2. Accuracy: score: 0. reason: The model's prediction for the next image's time is not accurate based on the pattern described in <P>. The model predicts 8:15, while the correct prediction based on <P> should be 7:40. 3. Specificity: score: 1. reason: Although the model's response is specific, it is not consistent with the pattern described in <P>. The times provided by the model do not match those given in <P>.

**MiniGPT-4:** The sequence shows a pattern of four images, from left to right, which represent the different stages of a product development process. The first image shows the initial conceptualization of the product, the second shows the prototype, the third shows the product in the market, and the fourth shows the product being used by customers. The pattern shows a logical progression of the product development process, starting with the initial idea and ending with the product being used by customers. The pattern shows that the product has been developed from a concept to a physical product and is now being used by customers. The fourth image shows the product being used by customers, which is the final stage of the product development process. This means that the product has been successfully developed

**GPT-4:** 1. LogicalConsistency: score: 0. reason: The model's response does not match the pattern described in <P>. The pattern in <P> is about a digital clock showing time increments of 10 minutes, but the model describes a product development process, which is completely irrelevant. 2. Accuracy: score: 0. reason: The model's prediction for the next image is not accurate based on the guidelines provided in <P>. The model does not mention anything about the digital clock or the time being 7:40, which is the expected content of the next image according to <P>. 3. Specificity: score: 0. reason: The model's response is not specific to the pattern described in <P>. It does not provide any details about the digital clock or the time increments, instead it talks about a completely different topic - product development.

**mPLUG-Owl:** The pattern observed in the images is that each one displays a progressive time, with the leftmost image showing a time of 7:55, the second one showing 8:00, the third one showing 8:05, and the fourth one showing 8:10. Based on this pattern, it can be predicted that the upcoming image will display a time of 8:15.

**GPT-4:** 1. LogicalConsistency: score: 1. reason: The model's response vaguely describes a timeline but does not specifically mention the pattern of the digital clock increasing by 10 minutes in each image. 2. Accuracy: score: 0. reason: The model does not predict the content of the next image based on the pattern described in <P>. It does not mention the time 7:40 which should be shown on the digital clock in the next image. 3. Specificity: score: 1. reason: The model's response is not specific to the pattern described in <P>. It does not provide a clear and concise pattern and future image, and it does not mention the digital clock or the time.

**InstructBLIP:** In this video, the content displayed changes according to a pattern of 7:00, 10:00, 13:00, 16:00, 19:00, 22:00, 25:00, and 01:00. It is likely that the video will continue to display the time in this pattern until it reaches the final time of 01:00, at which point the video will end.

**GPT-4:** 1. LogicalConsistency: score: 0. reason: The model's response does not match the pattern described in <P>. The pattern in <P> is a 10-minute increment in time, starting from 7:00, but the model describes a different pattern of time increments. 2. Accuracy: score: 0. reason: The model's prediction for the next image does not match the prediction given in <P>. The model predicts a time sequence that is not consistent with the 10-minute increment pattern described in <P>. 3. Specificity: score: 1. reason: The model provides a specific pattern and future image, but it is not consistent with the pattern described in <P>. The model's pattern involves a different time increment and also includes times that are not possible on a digital clock (25:00).

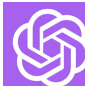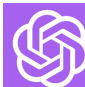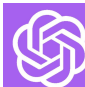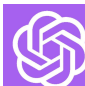

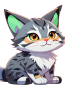

**Lynx:** the pattern is a sequence of images in which the image on the left is repeated three times, while the images on right are repeated twice. the upcoming image will be the fourth image in the sequence, which is the same image as the first image. this pattern will continue for a total of 12 images, with each image being repeated once.

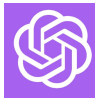

**GPT-4:** 1. LogicalConsistency: score: 0. reason: The model's response does not match the pattern described in <P>. The pattern is about the time shown on a digital clock increasing by 10 minutes in each image, but the model describes a completely different pattern involving a person, a car, a house, and a tree.

2. Accuracy: score: 0. reason: The model's prediction for the next image is completely unrelated to the pattern described in <P>. The model predicts an object related to nature, while according to the pattern, the next image should show a digital clock displaying the time 7:40.

3. Specificity: score: 0. reason: The model's response is detailed but not relevant to the pattern described in <P>. It provides a clear and concise pattern and future image, but it's about a completely different pattern involving a person, a car, a house, and a tree, not about the time on a digital clock.

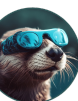

**Otter:** The video changes to show the time on a digital screen.

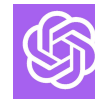

**GPT-4:** 1. LogicalConsistency: score: 1. reason: The model's response vaguely refers to a digital screen showing time, but it does not specifically mention the pattern of the time increasing by 10 minutes in each image, as described in <P>.

2. Accuracy: score: 0. reason: The model's response does not predict the content of the next image based on <P>'s guidelines. It does not mention that the next image will show the time as 7:40.

3. Specificity: score: 1. reason: The model's response is not specific or detailed. It does not provide a clear and concise pattern or future image, and it does not mention the specific time that will be shown in the next image.
